# Supplementary material for: Contact-Induced Semiconductor-to-Metal Transition in Single-Layer WS$_2$
Source: arXiv:1708.02799 ancillary file (2017-08-09)
Supplement: Supplementary file 1 [file WS2Ag_Supp9.pdf]

# Contact-induced semiconductor-to-metal transition in single-layer WS<sub>2</sub>: Supplementary Material

Maciej Dendzik, Albert Bruix, Matteo Michiardi, Arlette S. Ngankeu, Marco Bianchi, Jill A. Miwa, Bjørk Hammer, Philip Hofmann, and Charlotte Sanders\*

*Department of Physics and Astronomy, Interdisciplinary Nanoscience Center, Aarhus University, 8000 Aarhus C, Denmark*

E-mail: [sanders.charlotte@phys.au.dk](mailto:sanders.charlotte@phys.au.dk)

Phone: +45 871 55585. Fax: +45 861 20740

Figure S1 shows photoemission data for a clean Ag(111) surface, corresponding to the data for WS<sub>2</sub> on Ag(111) in Figure 2 of the main paper. The clean surface shows the surface state around  $\bar{\Gamma}$ ,<sup>1</sup> and more intensity in the projected bulk *sp* bands than is seen in Figure 2. The enhanced photoemission intensity observed at the Fermi level between  $\Gamma$  and *K* of the WS<sub>2</sub>/Ag(111) system is missing.

In order to study possible strain in SL WS<sub>2</sub>, we have analyzed spot positions in data acquired by low energy electron diffraction (LEED). We follow the procedure of Ref.<sup>2</sup> Figure S2 shows the actual LEED patterns together with line profiles through the first order spots of WS<sub>2</sub>, the first order spots of the substrate, and the moiré pattern, fitted with Lorentzians. The distance in reciprocal space is normalized such that outermost peak positions correspond to  $\pm 1$ , as seen in Fig. S2 (b),(d). In this way, the ratio of reciprocal lattice vectors of WS<sub>2</sub> and the substrate is directly given by the position of the middle peak. We use the

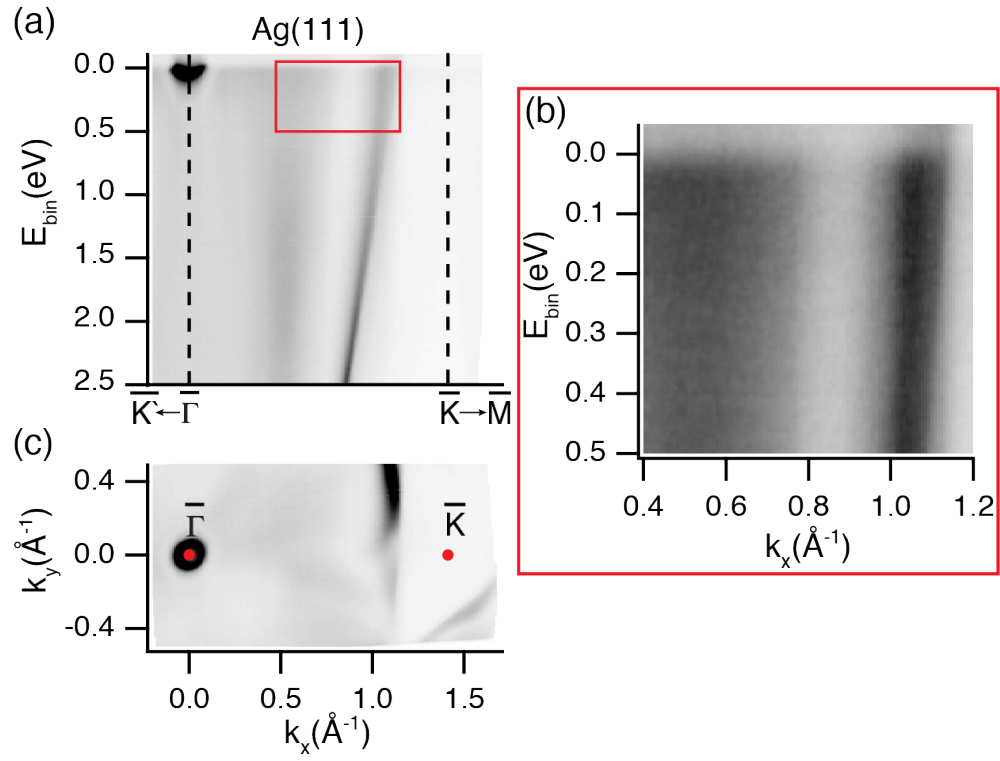

Figure S1: ARPES for clean Ag(111), corresponding to Figure 2 in the main paper ( $h\nu=25$  eV).

lattice constants of Au and Ag to calculate the lattice spacing of SL WS<sub>2</sub>. This procedure, performed for three equivalent cuts in reciprocal space and three images taken at different energies (in total, 36 data points) yields a lattice constant of 3.151(19) Å for WS<sub>2</sub>/Au(111) and 3.152(21) Å for WS<sub>2</sub>/Ag(111). These values are in excellent agreement with the bulk WS<sub>2</sub> lattice constant of 3.1532(4) Å.<sup>3</sup> Based on this analysis, we can exclude the possibility of strain larger than 0.7% for SL WS<sub>2</sub> grown on Ag(111) and Au(111).

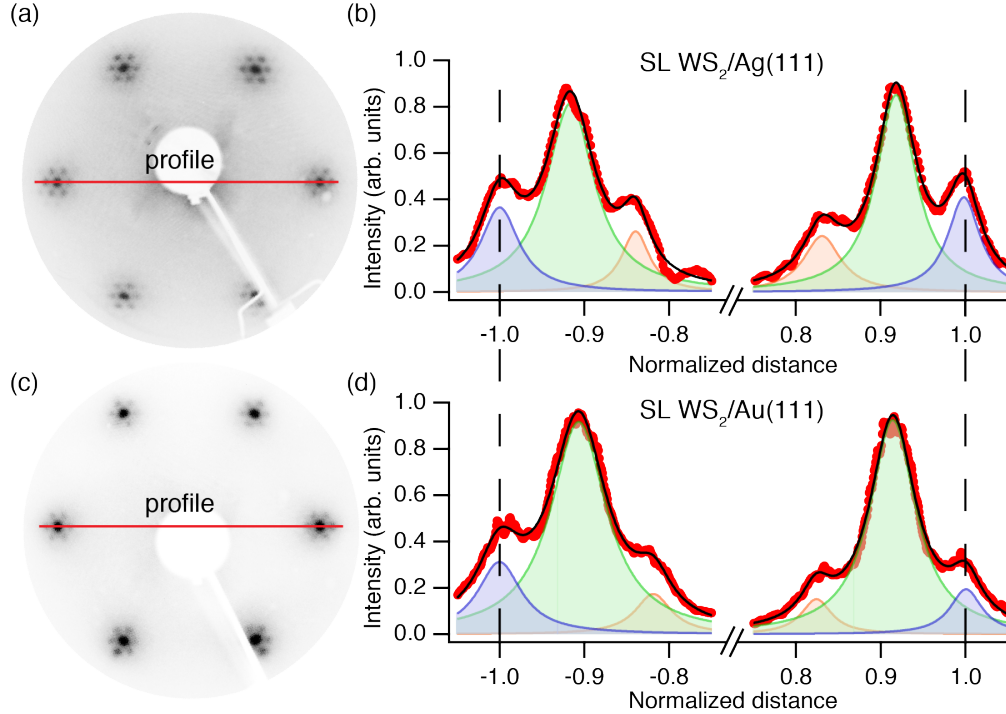

Figure S2: (a), (c) Comparison of LEED images taken with kinetic energy 114 eV for samples of  $\approx 0.75$  ML WS<sub>2</sub>/Ag(111) and WS<sub>2</sub>/Au(111), respectively. (b), (d) Line profiles through first order spots, as indicated in (a) and (c), respectively. The LEED intensity profiles (red points) are fitted with Lorentzian line shapes (colored curves) on a linear background. Black lines correspond to the sum of all peaks. Note that the WS<sub>2</sub> spots and moiré (green and orange curves) are slightly shifted for profiles in (b) and (d), consistent with the ca. 0.2% difference in lattice constant between Au and Ag.

Figures S3 and S4 give more information on the orbital character of the bands in free-standing WS<sub>2</sub>. Figure S3 shows a decomposition of all bands into the contributions of S and W orbitals, while Fig. S4 shows the contributions to the lowest lying conduction band in detail.

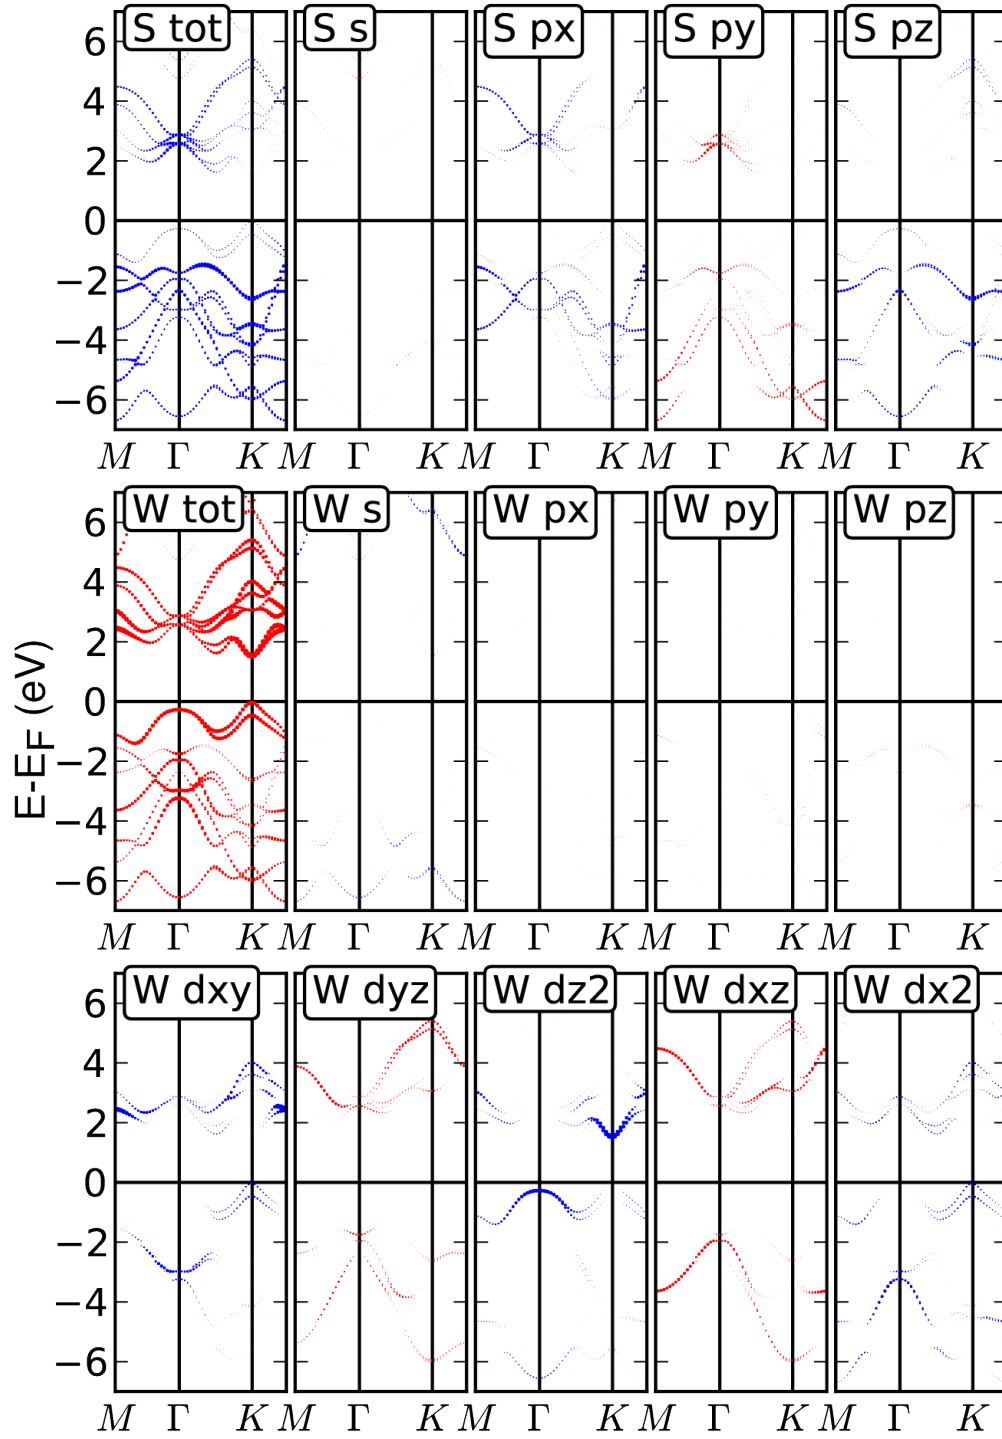

Figure S3: Calculated band structure of free-standing  $\text{WS}_2$ . The size of the data point for each eigenvalue is proportional to the contribution of the S or W orbital indicated in the plot. For the “S tot” and “W tot” plots the size of the points for each eigenvalue is proportional to the added weights of all orbitals of S and W, respectively.

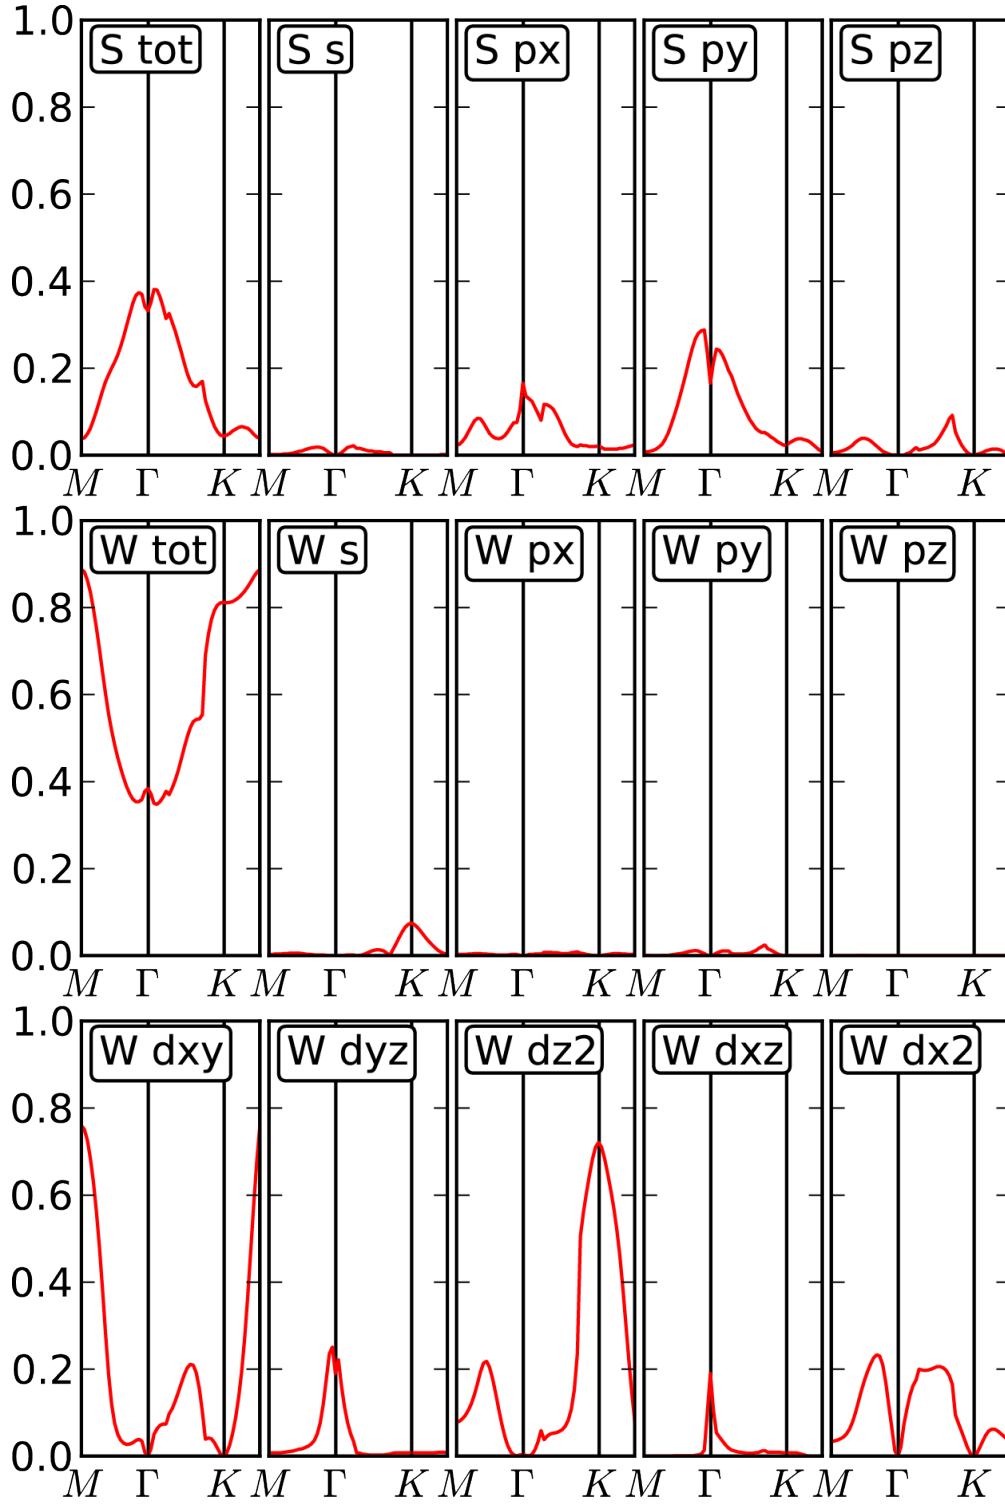

Figure S4: Contribution of each W and S orbital to the lowest-lying CB of free standing WS<sub>2</sub>. “S tot” and “W tot” correspond to added contributions of all orbitals of S and W, respectively.

Table 1 lists the absolute positions of the fitted peaks shown in Figure 1 of the main text. The main peaks, corresponding to the basal plane of WS<sub>2</sub>, were fitted using Doniach-Šunjić (DS) profiles convoluted with Gaussians. Aside from the asymmetry, the peak shape of the W 4*f* core levels for both WS<sub>2</sub>/Au(111) and WS<sub>2</sub>/Ag(111) is characterized by a Lorentzian width of ca. 0.19 eV and a Gaussian broadening of ca. 0.08 eV. We emphasize that the asymmetric lineshape for WS<sub>2</sub>/Ag(111) is the only viable option for a proper fit. The asymmetric long tail towards the high binding energy side cannot be fitted with an extra component.

Detailed analysis of the peaks corresponding to partially sulphided W is rather complex, due to the large number of contributions to such peaks at binding energies in this range—defects, for instance, and nanocluster edges.<sup>4</sup> We find this part of the core level spectrum to vary greatly for different samples depending on the WS<sub>2</sub> quality. However, intensity originating from the partially sulphided regions is much lower than from the basal plane, and we find it sufficient to fit this part of the spectrum with just a single Gaussian-broadened Lorentzian. The separation between main and secondary peak is ca. 0.2 eV—suggesting a trend similar to that observed previously in the closely related system MoS<sub>2</sub>/Au(111), where the reported separation was 0.4 eV.<sup>4</sup>

We assumed a linear background for fitting, because non-linear backgrounds can artificially decrease the asymmetry of the DS profile (this is especially true for the Shirley type of background, which is proportional to area under the fitted curve). Nevertheless, under the present experimental conditions ( $h\nu = 140$  eV) the intensity of W 4*f* core levels is excellent and the contribution from the background marginal. The different baselines observable for WS<sub>2</sub>/Au(111) and WS<sub>2</sub>/Ag(111) in Fig. 1 of the main text result from the long tail of the DS profile, and not from the background itself.

Table 1: Binding energies of peaks fitted to core-level spectra.

|                          | basal plane |            | partially sulphided |            |
|--------------------------|-------------|------------|---------------------|------------|
|                          | $4f_{5/2}$  | $4f_{7/2}$ | $4f_{5/2}$          | $4f_{7/2}$ |
| WS <sub>2</sub> /Ag(111) | 35.071(1)   | 32.921(1)  | 34.858(29)          | 32.721(14) |
| WS <sub>2</sub> /Au(111) | 34.857(1)   | 32.722(1)  | 34.658(10)          | 32.515(9)  |

## References

- (1) Nicolay, G. *et al.* Natural linewidth of the Ag(111) L-gap surface state as determined by photoemission spectroscopy. *Physical Review B* **62**, 1631–1634 (2000).
- (2) Ulstrup, S. *et al.* Manifestation of nonlocal electron-electron interaction in graphene. *Physical Review B* **94** (2016).
- (3) Schutte, W., De Boer, J. & Jellinek, F. Crystal structures of tungsten disulfide and diselenide. *Journal of Solid State Chemistry* **70**, 207 (1987).
- (4) Bruix, A. *et al.* *In Situ* Detection of Active Edge Sites in Single-Layer MoS<sub>2</sub> Catalysts. *ACS Nano* **9**, 9322 (2015).
